# Supplementary material for: A local Bayesian optimizer for atomic structures
Source: arXiv:1808.08588 ancillary file (2019-08-29)
Supplement: Supplementary file 1 [file SupplementaryMaterial.pdf]

# A local Bayesian optimizer for atomic structures
## Supplementary Material

Estefanía Garijo del Río, Jens Jørgen Mortensen, and Karsten Wedel Jacobsen
*CAMD, Department of Physics, Technical University of Denmark*

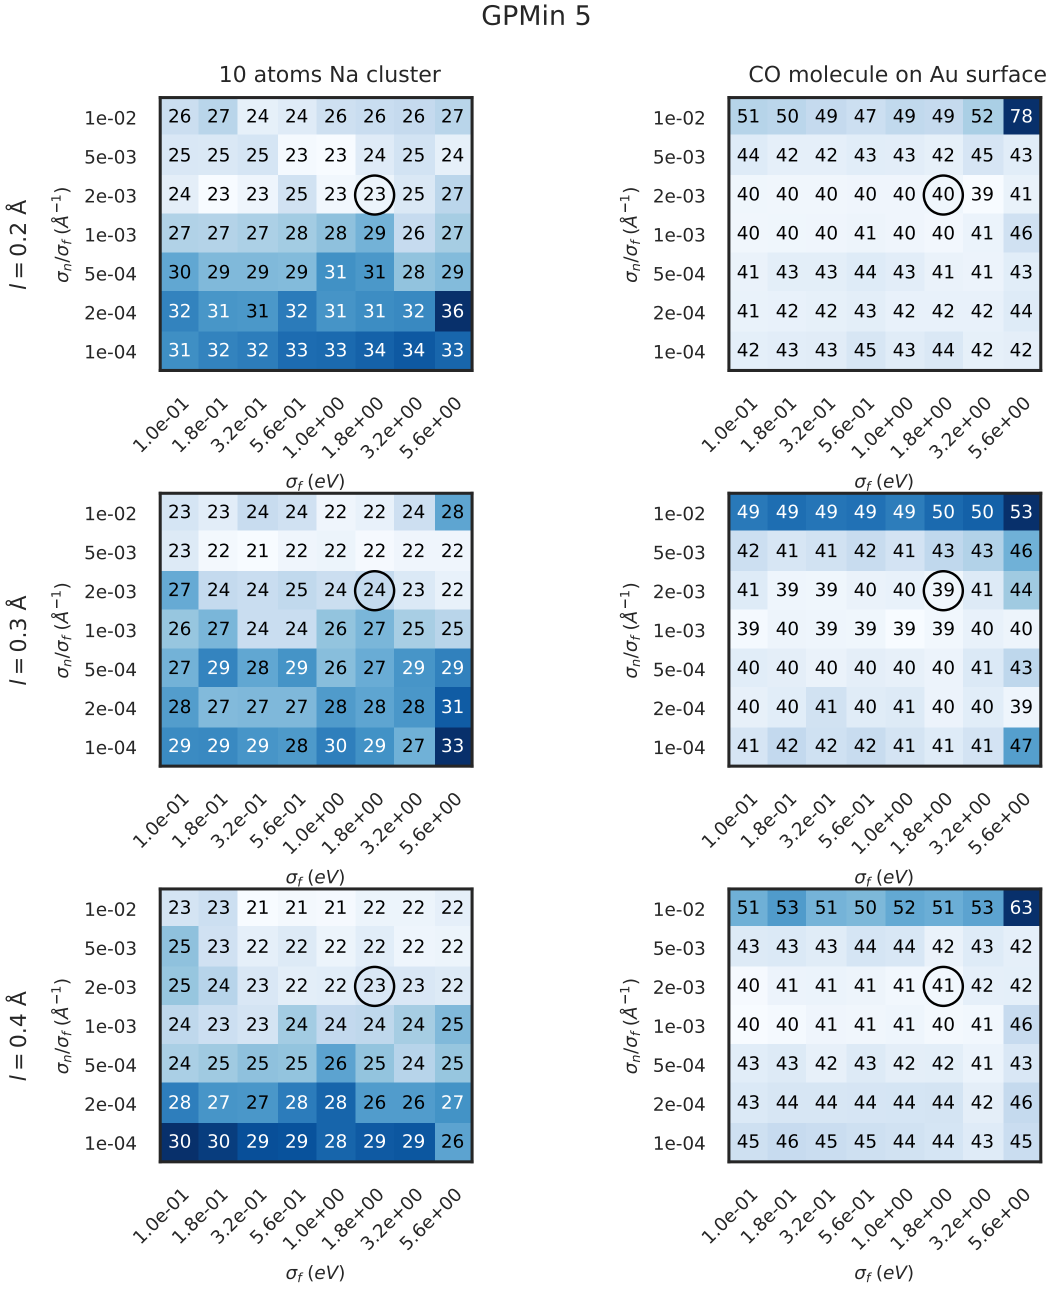


Figure S1. Average number of potential energy evaluations needed to relax 10 atomic structures with updated GPMin, using unconstrained optimization every $5^{\text{th}}$ step to optimize the marginal log-likelihood. The results are displayed as a function of the hyperparameters: the initial value of the length scale $l$, the initial value of the width $\sigma_f$, and the value of the regularization parameter $\sigma_n/\sigma_f$. The label NC (Not Converged) indicates that at least one of the relaxations did not converge. The default choice for the hyperparameters is indicated by a circle

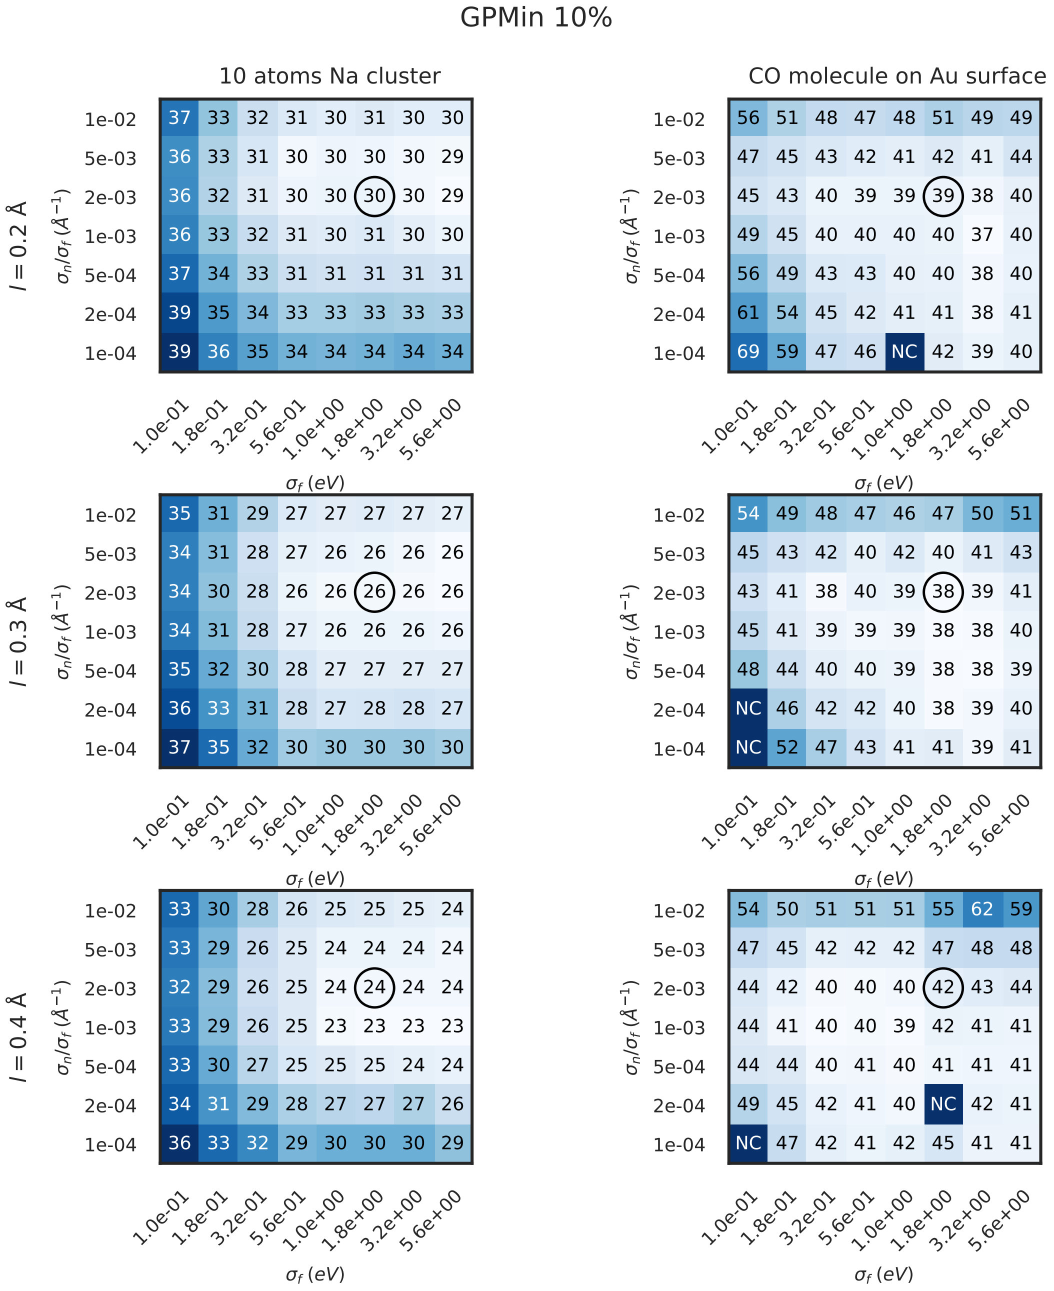


Figure S2. Average number of potential energy evaluations needed to relax 10 atomic structures with updated GPMin, using optimization constraint to 10% variation in the hyperparameters in every step to optimize the marginal log-likelihood. The results are displayed as a function of the hyperparameters: the initial value of the length scale $l$, the initial value of the width $\sigma_f$, and the value of the regularization parameter $\sigma_n/\sigma_f$. The label NC (Not Converged) indicates that at least one of the relaxations did not converge. The default choice for the hyperparameters is indicated by a circle

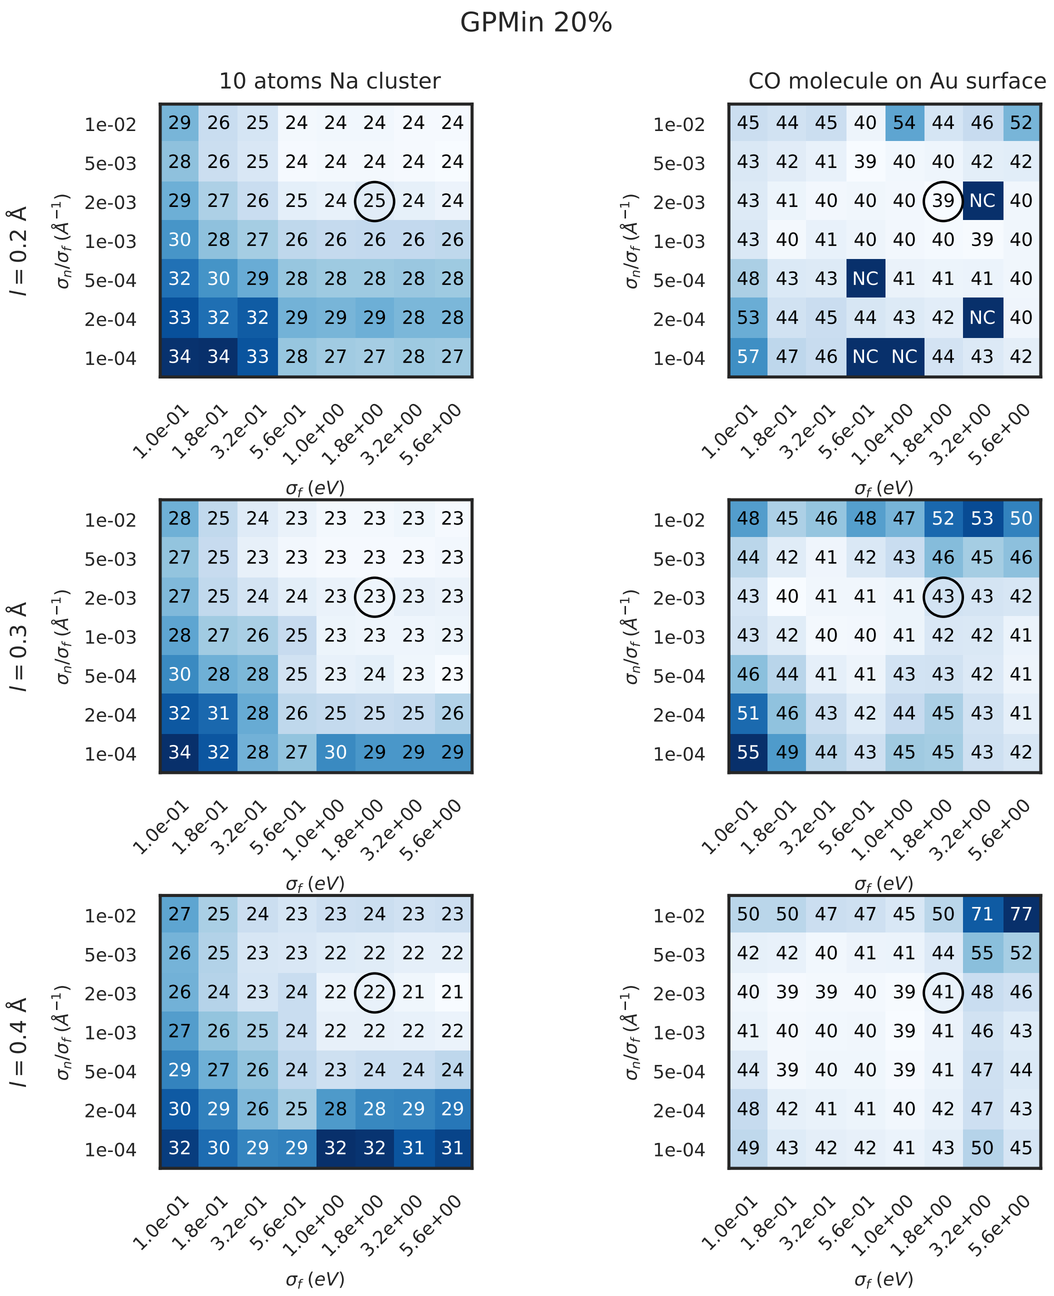


Figure S3. Average number of potential energy evaluations needed to relax 10 atomic structures with updated GPMin, using optimization constraint to 20% variation in the hyperparameters in every step to optimize the marginal log-likelihood. The results are displayed as a function of the hyperparameters: the initial value of the length scale $l$, the initial value of the width $\sigma_f$, and the value of the regularization parameter $\sigma_n/\sigma_f$. The label NC (Not Converged) indicates that at least one of the relaxations did not converge. The default choice for the hyperparameters is indicated by a circle

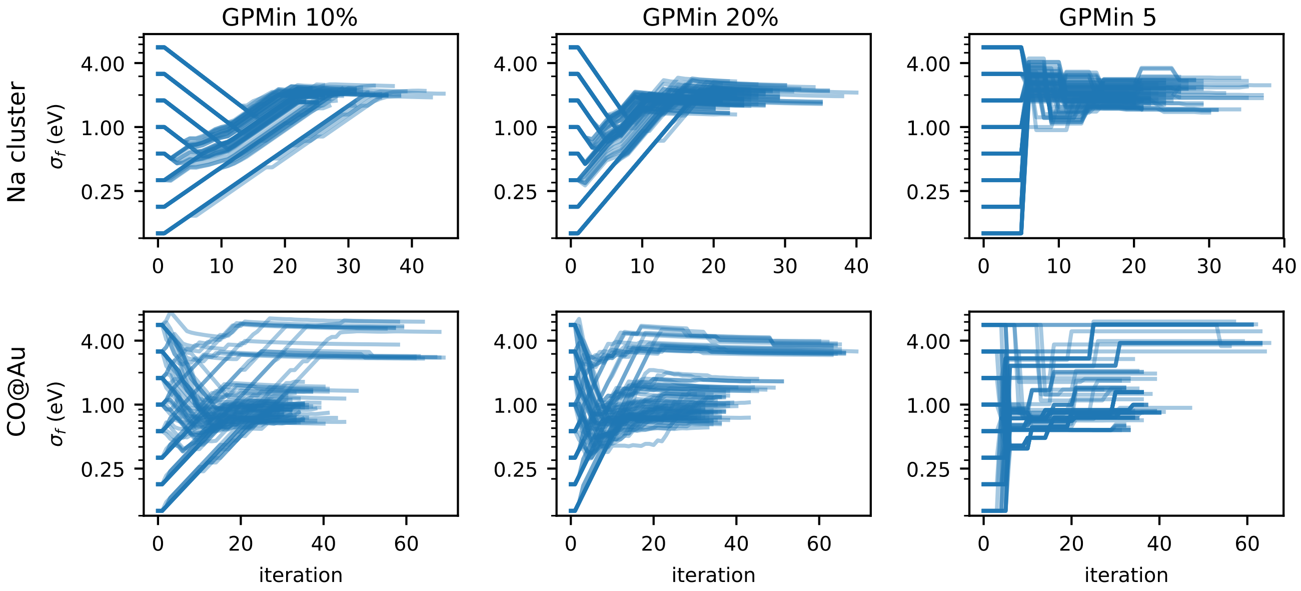


Figure S4. Evolution of $\sigma_f$ with the step in the updated GPMin. The plot shows the results for three different update strategies and for different initial values of $\sigma_f$.
